# Supplementary material for: Ancestral Inference from Functional Data: Statistical Methods and Numerical Examples
Source: arXiv:1208.0628 source file (2012-08-02)
Supplement: Supplementary file 1 [file SuppInfo.pdf]

# Supplementary Material : Ancestral Inference from Functional Data

Pantelis Z. Hadjipantelis, Nick, S. Jones, John Moriarty, David Springate, Christopher G. Knight

## Correlation matrix between true and estimated projection values

| | IPC est.1 | IPC est.2 | IPC est.3 |
|---|---|---|---|
| Real 1 | .989 / .908 | -.290 / -.154 | -.406 / -.297 |
| Real 2 | -.008 / .023 | .941 / .793 | -.038 / -.041 |
| Real 3 | -.396 / -.290 | .053 / .019 | .989 / .909 |

Table 1: Correlations between the true simulated weights (Real $i$) and the ones estimated using the PCA projection (PC est.$i$). The values before the slash correspond to the parametric Pearson correlation coefficient, the ones after to the non-parametric Kendall rank-correlation coefficient.

## Correlation matrix between true and estimated projection values by PCA

| | PC est.1 | PC est.2 | PC est.3 |
|---|---|---|---|
| Real 1 | -.897 / -.688 | -.441 / -.292 | -.016 / -.045 |
| Real 2 | -.017 / -.012 | .047 / .039 | .998 / .965 |
| Real 3 | -.679 / -.485 | .728 / .525 | -.091 / -.048 |

Table 2: Table quantifying the correlations between the true mixing coefficient and the ones estimated using the PCA projection. First value correspond to the parametric Pearson correlation coefficient, second value to the non-parametric Kendall rank-correlation coefficient.

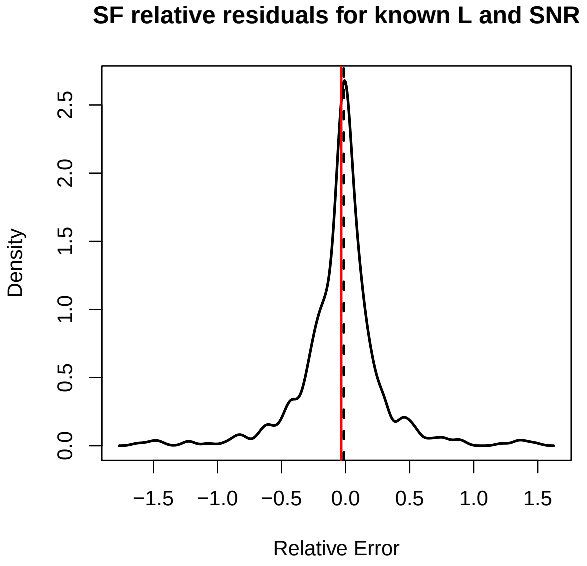


Figure 2: Kernel density estimates of the relative errors made during hyperparameter estimation when both $\lambda$ and the ratio between inherited and specific variation ($\sigma_f$ and $\sigma_n$ respectively) is known. $\lambda$ was drawn randomly from the interval [1,8]. The entire simulation was independently regenerated 512 times. The dashed black line indicates zero error, the red line the mean error across independent simulations.

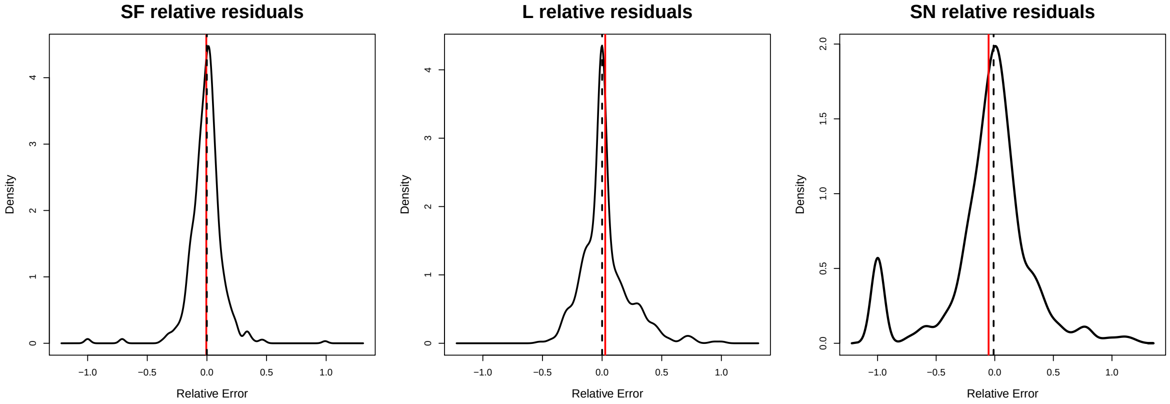


Figure 1: Kernel density estimates of the relative errors made during hyperparameter estimation. We fixed two of the three components of $\theta_i$ to random values, which were then assumed to be known *a priori*, and performed a numerical optimisation of the log-likehlihood in order to estimate the MLE of the third component, and recorded the relative error in this estimation. $\sigma_f$ was randomly drawn from the interval [.25,6], $\sigma_n$ from the interval [.25,1.5], and $\lambda$ from the interval [1,14]. The entire simulation was then independently regenerated 512 times. The dashed black line indicates zero error, the red line the mean error across independent simulations. The secondary bump in the right hand panel was caused when this penalised estimation fitted a lower dimensional model, setting $\sigma_n$ to zero with a consequent relative error of -1)
